# Supplementary material for: FISBe: A real-world benchmark dataset for instance segmentation of long-range thin filamentous structures
Source: arXiv:2404.00130 source file (2024-03-29)
Supplement: Supplementary file 1 [file preamble.tex]

%
% --- inline annotations
%
\usepackage[dvipsnames]{xcolor}
\newcommand{\red}[1]{{\color{red}#1}}
\newcommand{\todo}[1]{{\color{red}#1}}
\newcommand{\TODO}[1]{\textbf{\color{red}[TODO: #1]}}
% --- disable by uncommenting  
% \renewcommand{\TODO}[1]{}
% \renewcommand{\todo}[1]{#1}

\usepackage[ruled,vlined]{algorithm2e}
\usepackage{graphicx}
\usepackage{array}
\usepackage{subcaption}
\usepackage{dsfont}
\usepackage{tabu}
\usepackage{longtable}
\usepackage{listings}
\usepackage{multirow}
\usepackage{placeins}
\usepackage{tabularray}
\usepackage{afterpage}
\usepackage{float}
\usepackage[accsupp]{axessibility}
\UseTblrLibrary{booktabs}
\UseTblrLibrary{siunitx}
\NewColumnType{J}[1][]{Q[co=1,1.0,si={table-format=#1,table-number-alignment=center},c]}

\usepackage{siunitx}

\DeclareMathOperator*{\argmax}{arg\,max}
\DeclareMathOperator*{\argmin}{arg\,min}

\usepackage{tcolorbox}
\newtcbox{\revisedsec}[1][yellow]{on line, arc=0pt,colback=#1!100!white,colframe=#1!100!white,
  before upper={\rule[-3pt]{0pt}{10pt}},boxrule=1pt, boxsep=0pt,left=6pt,
  right=6pt,top=2pt,bottom=2pt}
\newcommand{\revised}[1]{\hl{#1}}

\newcommand{\subsubsubsection}[1]{\paragraph{#1}\mbox{}\\}
\setcounter{secnumdepth}{4}
\setcounter{tocdepth}{4}

\usepackage{soul}
\soulregister\cite7
\soulregister\ref7

\newcommand{\std}[1]{{\tiny$\pm$#1}}

 \lstset{
         language=Python,
         basicstyle=\footnotesize\ttfamily,
         %numbers=left,           
         %numberstyle=\footnotesize,       
         %numbersep=5pt,        
         tabsize=4,                 
         extendedchars=true,         
         breaklines=true,
         keywordstyle=\textbf,           
         stringstyle=\color{red}\ttfamily,
         showspaces=false,       
         showtabs=false,           
         xleftmargin=17pt,
         framexleftmargin=17pt,
         framexrightmargin=5pt,
         framexbottommargin=4pt,
         showstringspaces=false,
         upquote=true
 }

\usepackage[misc]{ifsym}
\usepackage{dblfloatfix}
\usepackage{multicol}
